# Supplementary material for: ChemFM as a Scaling Law Guided Foundation Model Pre-trained on Informative Chemicals
Source: arXiv:2410.21422 source file (2025-11-05)
Supplement: Supplementary file 1 [file ablation_studies.tex]

%\subsection{Ablation Studies}

\subsection{Ablation studies with different string representations and tokenizations}
\subsubsection{Molecule string representations}
\label{sec:ablation_study_molecule_string}
\subsubsection{Numerical representations and tokenizations}
\label{sec:ablation_study_numerical_value}

\begin{table}[h]
	\caption{\textbf{Performance comparison in property prediction task using different string representations and tokenizations.} \textcolor{red}{Just a placeholder}}
	\begin{tabular}{cccccc}
		
		\hline
		Molecule Encoding + Numerical Encoding & Validity $\uparrow$ & Uniqueness $\uparrow$ & Novelty $\uparrow$ & MAD $\downarrow$ & SD $\downarrow$\\
		%\hline
		%MolGPT & 0.972 & 0.998 & 0.967 & 0.054 & 0.050 \\ % this evaluation is rerun the molgpt code
		\hline
		%SMILES (less tokens) + Numerical Mapping  & 0.949 & 0.998 & 0.977 & 0.068 & 0.058 \\ % this smiles tokenizer is from the molgpt
		%SMILES (less tokens) + Numerical Mapping + Type Embedding  & 0.948 & 0.999 & 0.980 & 0.070 & 0.059 \\ % this smiles tokenizer is from the molgpt
		SMILES + Text Encoding & 0.959 & 0.999 & 0.975 & 0.060 & 0.054 \\ 
		SMILES + Numerical Mapping  & 0.951 & 0.999 & 0.978 & 0.066 & 0.059 \\
		%SELFIES + Numerical Mapping & 1.000 & 1.000 & 0.989 & 0.105 & 0.088 \\
		SMILES + Numerical Encoding & 0.949 & 0.999 & 0.979 & 0.063 & 0.056 \\
		SELFIES + Text Encoding & 1.000 & 1.000 & 0.985 & 0.094 & 0.080 \\
		\hline
	\end{tabular}
	\footnotetext{Mean average deviation (MAD), standard deviation (SD), validity, uniqueness, and novelty values for different encoding approaches in generation task; we use the single property ``QED" in GuacaMol dataset as an example.}
\end{table}
\begin{table}[h]
	\caption{\textbf{Performance comparison in generation task using different string representations and tokenizations.}}
	\begin{tabular}{cccccc}
		
		\hline
		Molecule Encoding + Numerical Encoding & Validity $\uparrow$ & Uniqueness $\uparrow$ & Novelty $\uparrow$ & MAD $\downarrow$ & SD $\downarrow$\\
		%\hline
		%MolGPT & 0.972 & 0.998 & 0.967 & 0.054 & 0.050 \\ % this evaluation is rerun the molgpt code
		\hline
		%SMILES (less tokens) + Numerical Mapping  & 0.949 & 0.998 & 0.977 & 0.068 & 0.058 \\ % this smiles tokenizer is from the molgpt
		%SMILES (less tokens) + Numerical Mapping + Type Embedding  & 0.948 & 0.999 & 0.980 & 0.070 & 0.059 \\ % this smiles tokenizer is from the molgpt
		SMILES + Text Encoding & 0.959 & 0.999 & 0.975 & 0.060 & 0.054 \\ 
		SMILES + Numerical Mapping  & 0.951 & 0.999 & 0.978 & 0.066 & 0.059 \\
		%SELFIES + Numerical Mapping & 1.000 & 1.000 & 0.989 & 0.105 & 0.088 \\
		SMILES + Numerical Encoding & 0.949 & 0.999 & 0.979 & 0.063 & 0.056 \\
		SELFIES + Text Encoding & 1.000 & 1.000 & 0.985 & 0.094 & 0.080 \\
		\hline
	\end{tabular}
	\footnotetext{Mean average deviation (MAD), standard deviation (SD), validity, uniqueness, and novelty values for different encoding approaches in generation task; we use the single property ``QED" in GuacaMol dataset as an example.}
\end{table}
