# Supplementary material for: ChemFM as a Scaling Law Guided Foundation Model Pre-trained on Informative Chemicals
Source: arXiv:2410.21422 source file (2025-11-05)
Supplement: Supplementary file 2 [file appendices.tex]

\begin{appendices}
	\section{Section title of first appendix}\label{secA1}
\end{appendices}
